# Supplementary material for: Mathematical foundations for symmetric programming and reasoning
Source: arXiv:2611.17106 source file (2026-11-12)
Supplement: Supplementary file 1 [file bst.tex]

\section{Case study II: Binary search trees}
\applabel{bst}

We now develop an extended case study using binary search
trees~(BSTs), demonstrating all the concepts we have developed so far.

We proceed as follows. In \subsecref{bst:aux} we introduce auxliary
indexed families and their actions that will serve the remainder.  In
\subsecref{bst:core} we introduce the main indexed family of interest,
that of BSTs, following \citepos{mcbride:neighbours-in-order} design
to store key comparisons in the leafs of the tree.  In
\subsecref{bst:insert}, we demonstrate how to insert a key into a BST
using wlog. In \subsecref{bst:discuss} we discuss lessons we learned
during this use case.

\subsection{Auxiliary data}
\subseclabel{bst:aux}
Our goal is to address the $\Sym2$-symmetry inherent in BSTs. We
therefore adapt \citepos{mcbride:neighbours-in-order} auxiliary
concepts and define indexed actions over them.

One of the subtleties in the development, that we will deal with on an
ad-hoc basis, is that most constructions will require us to
\emph{propagate} an action. For example, homogeneous pairs
$\A\times\A$ have a $\Sym 2$-action given by \emph{shallow} swapping
$\swap\act\pair{a}{b} \definedby \pair ba$. But often we will need to
propagate an action on $\A$ in the form of \emph{deep swapping}
$\swap\act\pair{a}{b} \definedby \pair{\swap \act b}{\swap \act
  a}$. For the data types in \secref{algebraic data types}, we used the
symmetry strength. Indexed data types ought to have a similar notion
of symmetry strength, but an comprehensive theory of initial algebra
semantics for indexed data types is still an open problem. We will
therefore carefully introduce the relevant actions and explicitly
choose the appropriate one in each situation.


Fix a set $\keys$ of \emph{keys}, equipped with the trivial action.
Consider the set of \emph{decidable
total ordering functions} over $\keys$:
\begin{multline*}
\Total[\keys] \definedby
\DPair{(\prelt)}{\Fun{\keys^2}\Prop}\\
\DPair{\cmp}{\DFun{(\x,\y)}{\keys^2}
  (\LT : \x \prelt \y) \Or (\EQ : \x = \y) \Or (\GT : \y \prelt \x)}
\\\parent{(\prelt) \text{ irreflexive and transitive}}
\end{multline*}
The product $\keys^2$ has an action structure given by $\swap \act
(a,b) \definedby (b,a)$. This action is both the deep and shallow
swapping action, as they coincide when we use the trivial action on
$\keys$. We use the action exponential to derive the action on
$\Rel\keys \definedby \Fun{\keys^2}\Prop$ given by $\swap \act
(\prelt) \definedby (\pregt) \definedby \fun{\pair ab} b \prelt a$.
We will overload notation and refer to their first component of
$\Total[\keys]$ elements $(\prelt)$ by $(\prelt)$ as well.

Let $\A$ be a $\Ctx$-indexed $\Sym 2$-action, and consider an
invariant proposition $\Ctx, (\x,\y) : \A^2 \types P(\x,\y) :
\Prop$. We then have an indexed $\Sym 2$-action $\Ctx, (\x,\y) : \A^2
\types P(\x,\y)$.  We define an indexed action on the following
\emph{trichotomy} family, using the deep swapping action on $\A^2$:
\begin{gather*}
  \begin{aligned}[t]
    \Ctx,((\x,\y) : \A^2)\types{}
    & \trichotomy P \definedby \\
    & (\LT : P(\x,\y)) \\
    \Or {}& (\EQ : \x = \y) \\
    \Or {}& (\GT : P(\y,\x))
  \end{aligned}
\qquad
\begin{aligned}[t]
    \stet \act{}& x \definedby x
    \\
    \swap \act{}& \LT (p : P_{\ctx}(\x,\y)) \definedby
    \GT (\swap \act p : P_{\swap\act\ctx}(\swap \act \y, \swap \act \x))
    \\
    \swap \act{}& \EQ (p : \x = \y) \definedby
    \EQ (p : \swap \act \y = \swap \act \x)
    \\
    \swap \act{}& \GT (p : P_{\ctx}(\y,\x)) \definedby
    \LT (\swap \act p : P_{\swap\act\ctx}(\swap \act \x, \swap \act \y))
  \end{aligned}
\end{gather*}
Using \exampleref{indexed function space action}, we obtain an indexed action
over the family:
\[
((\prelt) : \Rel\keys)\types
\DFun{(\x,\y)}{\keys^2}(\LT : \x \prelt \y) \Or (\EQ : \x = \y)
\Or (\GT : \y \prelt \x)
\]
Note that the properties `irreflexive' and `transitive' are invariant
functions $\Rel\keys \equito \Prop$, and so their conjunction is
invariant and, by \exampleref{schur's inequality actions}, becomes an
indexed action. Putting these together, using \exampleref{extension
  and dpair action}, we have an $\Sym2$-action over $\Total[\keys]$.

We formally add extrema to the set of keys, and the action flips them:
\[
\Sandwich\keys \definedby
\keys \Or \set{\pminfty}
\qquad
\swap \act \pminfty \definedby \mpinfty \qquad
g \act a \definedby a
\]
We can lift any relation on $\keys$ to one on $\Sandwich\keys$, making
$\pminfty$ extrema, and this lifting is equivariant:
\[
\sandwich- : \EFun{(\prelt)}{\Rel\keys} \Rel(\Sandwich\keys)
\qquad
x \sandwich\prelt y \definedby \begin{cases}
  x = \minfty, y \neq \minfty: & \Tru \\
  x \neq \pinfty, y = \pinfty: & \Tru \\
  x,y \neq \pminfty: & x \prelt y \\
  \text{otherwise}: & \Fls
\end{cases}
\]
We prove equivariance by currying the equivariant term
$(\prelt) : \Rel \keys, (\x,\y) : (\Sandwich\keys)^2 \types \x
\sandwich\prelt \y$. To show the equivariance of the latter, we could
use wlog to deal with the top two cases symmetrically. In our
view it is not worth the hassle, we show that
$(\swap \act y)\sandwich\pregt (\swap \act x) = x
\sandwich\prelt y$ by a straightforward calculation,
taking care not confuse $(\sandwich\pregt)$ with
$(\sandwich{}\pregt)$. Indeed:
\[
\begin{cases}
  x = \minfty, y \neq \minfty: &  (\swap \act y)\sandwich\pregt (\swap \act x)
  = (\swap\act y) \sandwich\pregt \infty = \Tru = x \sandwich\prelt y \\
  x \neq \pinfty, y = \pinfty: & (\swap \act y)\sandwich\pregt (\swap \act x)
  = \minfty \sandwich\pregt (\swap\act x) = \Tru
  = x \sandwich\prelt y
  \\
  x,y \neq \pminfty: & (\swap \act y)\sandwich\pregt (\swap \act x)
  = y \sandwich\pregt x = y \pregt x = x \prelt y
  = x \sandwich\prelt y
  \\
  \text{otherwise}: & (\swap \act y)\sandwich\pregt (\swap \act x)
  = \Fls
  = x \sandwich\prelt y
\end{cases}
\]
Given $(\prelt) : \Rel\keys$ and a $\cmp$ function for it, we can
construct the function $\sandwich\cmp$ for $\sandwich\prelt$. Here
it will be useful to use wlog reasoning, although we will not require
the equivariance of the comparison function. The canoniser will eliminate
the two cases where $\x \neq \pminfty$ but $y = \pminfty$:
\[
  \canoniser(\pminfty, y) \definedby \stet\qquad
  \canoniser(x, \pminfty) \definedby \swap\quad
  \canoniser(x,y) \definedby \stet
\]
The canonical elements are then
$\set{\pair\pminfty\pminfty, \pair\pminfty y, \pair xy \suchthat x,y \in \keys}$.
We can then define:
\[
f(\minfty, \minfty) \definedby \EQ \star
\quad
f(\minfty, x) \definedby \LT \star
\quad
f(x, y) \definedby \cmp\pair xy
\qquad
\sandwich\cmp \definedby \wlg(c,f)
\]
For example, for $a \in \keys$ and recalling the trichotomy action, we have:
\[
\sandwich\cmp\pair{a}{\pinfty} =
\swap \act f\pair{\minfty}{a} =
\swap \act\LT(\star : \minfty \sandwich\pregt a) =
\GT(\star : a \sandwich\prelt \infty)
\]
and so $\sandwich\cmp$ is defined as expected.  Since
$(\sandwich\prelt)$ is irreflexive and transitive when $(\prelt)$ is,
we can lift $\sandwich-$ to a function $\sandwich- : \Total[\keys] \to
\Total[\Sandwich\keys]$. The third component of this function is an
equivariant property. Given irreflexivity and transitivity, the
comparison map is unique, and therefore equivariant. Therefore we have
an equivariant function $\sandwich- : \Total[\keys] \equito
\Total[\Sandwich\keys]$.
%
An \emph{open interval} over $\keys$ is a pair of elements
$\interval[\keys] \definedby (\Sandwich\keys)^2$. The $\Sym 2$-action
on it is the deep swapping action. Each interval encodes an indexed
action over the family of elements inside that interval:
\[
(\prelt) : \Total[\keys], (\x,\y) : \interval[\keys] \types (\x,\y)
\quad
(\x,\y)_{(\prelt), \For{(\x,\y)}(a,b)} \definedby \set{k \in \keys \suchthat a \sandwich\prelt x \sandwich\prelt b}
\quad
g\iact*{(\prelt), (a,b)} k \definedby k
\]

\subsection{Core data}
\subseclabel{bst:core} We now define the core data structure: binary
search trees.  For convenience, let $\Btx$ be the indexing set
$(\prelt) : \Total[\keys], (\x,\y) : \interval[\keys]$.  We define
inductively the family of \emph{binary search trees} $\Btx \types \BST\prelt{(\x,\y)}$:
\[
\inferrule{
  p : a \sandwich\prelt b
}{
  \TLeaf[p] : \BST\prelt{(a,b)}
}
\qquad
\inferrule{
  \ell : \BST\prelt{(a,x)}
  r    : \BST\prelt{(x,b)}
}{
  \TNode x\ell r : \BST\prelt{(a,b)}
}
\]
We characterise this family as an initial algebra for the
following functor over $\Btx$-families and their vertical maps:
\begin{gather*}
\structBST(\Btx \types \X)_{(\prelt), (a,b)} \definedby
\TLeaf[a \sandwich \prelt b] \Or
\TNode[] \DPair\x\keys\Pair{\X_{(\prelt), (a, \x)}}{\X_{(\prelt), (\x, b)}}
\qquad
\fmap[\structBST]f\TLeaf[p] \definedby \TLeaf[p]
\\
\fmap[\structBST]f\NodeV {\ell : \X_{(\prelt), (a,x)}}x{r : \X_{(\prelt), (x,b)}}
\definedby \NodeV {f_{(\prelt), (a,x)}\ell}x{{f_{(\prelt), (x,b)}r}}
\tag{$\Btx \types f : \X \to \Y$}
\end{gather*}
\begin{proposition}
  The $\Btx$-indexed family of binary search trees is the initial
  $\structBST$-algebra.
\end{proposition}
For every $\structBST$-algebra $\Btx \types \coseq{\tleaf,\tnode} :
\structBST\X \to \X$, the unique $\structBST$-homomorphism into it is the
following unique vertical map $\Btx \types \fold\coseq{\tleaf,\tnode} : \BST{\prelt}{(\x,\y)} \to \X$ satisfying:
\begin{gather*}
\fold\coseq{\tleaf,\tnode}\TLeaf[p] \definedby \tleaf p
\\
\fold\coseq{\tleaf,\tnode}\NodeV {\ell : \X_{(\prelt), (a,x)}} x {r : \X_{(\prelt), (a,x)}} \definedby \tnode\triple x\ell r
\end{gather*}


Define the following natural transformation over $\Btx$-indexed
families and vertical morphisms:
\begin{gather*}
\strength : \gast[\Sym2] \structBST \X \to
\structBST\parent{\gast[\Sym2]\X}
\qquad
\strength\pair\stet t \definedby \fmap(\fun x\pair\unit) x
\\
\strength\pair\swap {\TLeaf[p : b \sandwich\pregt a]}
\definedby \TLeaf[\swap \act p : a \sandwich\prelt b] :
\parent{\structBST\parent{\gast[\Sym2]\X}}_{(\prelt), (a,b)}
\\
\strength\pair\swap
          {\NodeV {r : \X_{(\pregt), (b,x)}}n{\ell : \X_{{\pregt}{(x,a)}}}}
\definedby
\begin{array}[t]{@{}l@{}}
  \NodeV{\pair\swap{\ell}}x{\pair\swap{r}}
    \\
    \qquad: \parent{\structBST\parent{\gast[\Sym2]\X}}_{(\prelt), (a,b)}
\end{array}
\end{gather*}
\begin{proposition}\propositionlabel{bst strength is strength}
  This strength is a $\Sym2$-symmetry strength in the sense of
  \definitionref{indexed symmetry strength}.
\end{proposition}

By the Indexed Equivariant Initiality \theoremref{indexed representation}, we
have an indexed action over binary search trees. For leafs:
\(
\swap \iact*{(\prelt), (a,b)}\TLeaf[p] =
\roll \compose \fmap(\act)\compose \strength(\swap, \TLeaf[p]) \definedby
\TLeaf[\swap \act p]
\), and nodes:
\begin{align*}
\swap \iact{(\prelt), (a,b)}&\NodeV \ell n r
\roll \compose \fmap(\act)\compose \strength(\swap, \NodeV \ell n r)
\\&\definedby
\roll \compose \fmap(\act)(\NodeV{\pair\act r}n{\pair\swap\ell})
=
\NodeV{\swap \act r}n{\swap\act \ell}
\end{align*}
as one might expect. We will now use this symmetry to define
operations over binary search trees.

\subsection{Insertion}
\subseclabel{bst:insert}
Our goal is to define the following dependent function:
\[
\insrt :
\DFun{(\prelt)}{\Total}
\DFun\mk\keys
\DFun{(\x,\y)}{\interval[\keys]}
\Fun{\x \sandwich\prelt \mk \sandwich\prelt \y}
\Fun{\BST{\prelt}(\x,\y)}
\BST{\prelt}(\x,\y)
\]
To insert a key $k$ into a BST node, we need to insert it inductively
into the correct subtree, and keep the other subtree as is, or keep
the node as is if the key coincides with the root. We therefore need retain
both input tree and the recursive call. We will therefore use the following
indexing set and family as carrier for our $\structBST$-algebra:
\[
\Ctx \definedby (\prelt):\Total, \mk:\keys, (\x,\y):\interval[\keys]
\types
\qquad
\A \definedby\Pair{\BST[]{}{}}\A_2
\qquad
\A_2 \definedby
\Fun{\x \sandwich\prelt \mk \sandwich\prelt \y}
\BST{\prelt}(\x,\y)
\]
With the auxiliar and core constructs of the preceding two sections,
we have canonical actions on $\Ctx$, $\A_2$ and $\A$. Appealing to the
Indexed Equivariant Initiality \theoremref{indexed representation}, it
suffices to define an equivariant $\structBST$-algebra $\insrtElim :
\structBST\A \equito \A$, and then define:
\[
\insrt(\prelt)\, \mk\, (\x, \y)\, p\,t \definedby
(\projection_2(\fold \insrtElim\, t))_{(\prelt)\, \mk\, (\x, \y)}\,p
\]
which amounts to defining the two component functions equivariantly:
\[
\insrtElim_1 \structBST \A \xto{\fmap \projection_1} \structBST{\BST[]{}{}}
\xto\roll \BST[]{}{}
\qquad
\curry\insrtElim_2 : \structBST \A \equito
\Fun{\x \sandwich\prelt \mk \sandwich\prelt \y}
\BST{\prelt}(\x,\y)
\]
The first component reconstruct the input tree.  The second component
is the curried equivariant function which, given the top constructor
of a binary search tree with the results of the appropriate inductive
calls, will insert the key. It is this component we will define using
wlog reasoning. Define the canoniser:
\[
\canoniser : \carrier{\structBST\A} \to \Sym2
\qquad
\canoniser\, \Leaf \definedby \stet
\qquad
\canoniser \parent{\NodeV{u}n{v}} \definedby
\begin{cases}
  k \sandwich\prelt n \lor k = n: & \stet \\
  k \sandwich\pregt n: & \swap
\end{cases}
\]
Thus, the canonical elements are either $\Leaf$ or a node whose key is
not greater than $k$. Note that this canoniser is not
equivariant. When the node key is $n = k$, we have:
\[
\canoniser(\swap \act \NodeV{u}{k}{v})
=
\canoniser(\NodeV{\swap \act v}{k}{\swap \act u})
=
\stet
\not\stabeq{}
\swap
=
\stet \mul \inv\swap
=
\swap\act \canoniser(\NodeV{u}{k}{v})
\]
We define the following core function $\insrtCore : \Canon\canoniser \to \BST\prelt(\x,\y)$.
For leafs, remembering we have a proof that $a \sandwich\prelt k \sandwich\prelt b$
in context:
\[
\insrtCore \TLeaf \definedby
\NodeV {\displaystyle\TLeaf[\unitval : a\sandwich\prelt k]}k
       {\displaystyle\TLeaf[\unitval : k\sandwich\prelt b]}
\]
For nodes, we split into cases, remembering that for canonical elements
$k = n$ or $k \sandwich\prelt n$:
\[
\insrtCore \NodeV{\pair \ell{\rec_{\ell}}}n{\pair r{\rec_{r}}} \definedby
\begin{cases}
  k = n:               & \hfill\NodeV \ell nr\\
  k \sandwich\prelt n: & \NodeV {\rec_{\ell}(\unitval : a \sandwich\prelt k \sandwich\prelt n)}n r
\end{cases}
\]
This canoniser is equivariant. The only interesting case is when $k = n$.
In that case we have the two canonical eleements:
\[
\NodeV unv \qquad
\swap \act \NodeV unv = \NodeV{\swap\act v}n{\swap\act u}
\tag{
  where $u = \pair\ell{\rec_{\ell}}$, $v = \pair r{\rec_{r}}$
}
\]
We then have the $\insrtCore$ is indeed equivariant:
\[
\insrtCore(\swap \act \NodeV unv) =
\NodeV{\swap\act v}n{\swap\act u}=
\swap\act \insrtCore(\NodeV unv)
\]
Putting it all together, we define:
\[
\Ctx,\x \sandwich\prelt \mk \sandwich\prelt \y \types
\insrtElim_2 \definedby \wlg(\canoniser, \insrtCore)
: \structBST \A \equito \BST{\prelt}(\x,\y)
\]

\begin{proof}[\propositionref{bst strength is strength}]%
  For naturality, take any vertical map $\Btx \types f : \X \to \Y$
  and split into cases. To deal with the $\TLeaf[p]$ case, first note, by
  checking both cases $g = \stet,\swap$,
  that $\strength(g, \TLeaf[p]) = \TLeaf[g \act p]$. Now calculate:
  \begin{align*}
  \strength(g, \fmap[\structBST] f \TLeaf[p])
  &=
  \strength(g, \TLeaf[p])
  =
  \TLeaf[g \act p]
  =
  \fmap[\structBST] (\DPair\g\G{\g \act f}) \TLeaf[g \act p]
  \\&=
  \fmap[\structBST] (\DPair\g\G{\g \act f}) \compose \strength(g, \TLeaf[p])
  \end{align*}

  For $g = \stet$:
  \begin{align*}
    \strength&(\stet, \fmap f
    \NodeV{\ell : \X_{(\prelt), (a,b)}}x{r : \X_{(\prelt), (a,b)}})
    \\&=
  \strength(\stet,
  \NodeV{f\,\ell}x{f\,r})
  =
  \fmap\pair\stet-(\NodeV{f\,\ell}x{f\,r})
  \\&=
  \NodeV{\pair\stet{f\,\ell}}x{\pair\stet{f\,r}}
  \\&=
  \fmap (\DPair\g\G{\g \act f}) \compose \strength(\stet,
  \NodeV{\ell}x{r})
  \end{align*}
  For $g = \swap$:
  \begin{align*}
    \strength&(\swap, \fmap f
    \NodeV{\ell : \X_{(\prelt), (a,b)}}x{r : \X_{(\prelt), (a,b)}})
    \\&=
    \strength(\swap,
    \NodeV{f\,\ell}x{f\,r })
    =
    \NodeV{\pair\swap{f\,r }}x{\pair\swap{f\,\ell}}
  \\&=
  \fmap (\DPair\g\G{\g \act f}) (\NodeV{\pair\swap r}x{\pair\swap \ell})
  \\&=
  \fmap (\DPair\g\G{\g \act f}) \compose \strength(\swap,
  \NodeV{\ell}x{r})
  \end{align*}
  and so $\strength$ is natural.

  By definition, we have
  \(
  \strength\pair\stet{t} = \fmap (\fun x\pair\stet x) t
  \).
  We need to show that:
  \[
  \strength_{\X}(g\mul h, t)
  =
  \fmap[F] (\fun{\triple{g'}{h'}{x}}\pair{g'\mul h'}x)
  (\strength_{G\times\X}(g,
   \strength_{\X}(h, t)))
   \]

  By \lemmaref{indexed check only non-trivial},
  we need only for the case $g = h = \swap$.
  First, for leafs:
  \begin{align*}
    \fmap&(\mapmul)
  (\gstrength(\swap,
   \gstrength(\swap, \TLeaf[p])))
   =
   \fmap(\mapmul)
  (\gstrength(\swap,
   \TLeaf[\swap\act p]))
   \\&=
   \fmap(\mapmul)
   \TLeaf[\swap\act\swap\act p]
   =
   \TLeaf[\swap\act\swap\act p]
   =
   \gstrength(\swap\mul\swap, \TLeaf[p])
  \end{align*}
  For nodes:
  \begin{align*}
    \fmap&(\mapmul)
  (\gstrength(\swap,
   \gstrength(\swap, \NodeV{\ell : \X_{(\prelt), (a,x)}}x{r : \X_{(\prelt), (x,b)}})))
   \\&=
   \fmap(\mapmul)
  (\gstrength(\swap,
   \NodeV{\pair\swap r}x{\pair\swap\ell}))
   \\&=
   \fmap(\mapmul)
   (\NodeV{\pair\swap{\pair\swap r}}x{\pair\swap{\pair\swap\ell}})
   =
   (\NodeV{\pair{\swap\mul\swap}r}x{\pair{\swap\mul\swap}\ell})
   \\&=
   (\NodeV{\pair\stet r}x{\pair\stet\ell})
   = \gstrength(\stet,
   \NodeV{\ell}x{r})
= \gstrength(\swap\mul\swap,
   \NodeV{\ell}x{r})
  \end{align*}
  and so the indexed version of the second strength axiom holds.
\end{proof}
