# Supplementary material for: Mathematical foundations for symmetric programming and reasoning
Source: arXiv:2611.17106 source file (2026-11-12)
Supplement: Supplementary file 2 [file dag.tex]

\subsection{Directed acyclic graphs}
\subseclabel{directed-acyclic-graphs}

A more substantive example exhibiting symmetry are directed
acyclic graphs (DAGs), where one often presupposes that its vertices
are topologically sorted~\cite[Sec.~20.4]{cormen}, i.e. ordered in
such a way that all the edges go only forwards. Before seeing how the
\WLOG construction can formalise this assumption, let us recall a few
standard definitions.

Recall that every group $\G$ acts on every set $\X$ with the
\emph{trivial} action $\Triv \X$, defined by
  \(
    \carrier{\Triv \X} \definedby \X
  \) and \(
    g \act x \definedby x
  \)
  for all $g \in \carrier\G$.
  Recall that an \emph{invariant} map is an equivariant map $f : \A \equito \Triv
  \X$, i.e. $f (g \act a) = f a$ for all $g \in \carrier G$ and $x \in
  \carrier A$.
  Also recall that their \emph{exponential} $\A \to \B$ has as carrier
  the set of all functions
  \(
    \carrier{\A \to \B}\definedby \carrier\A \to \carrier\B
  \), not only the equivariant ones. Its action is given by
  \(
    (g \act \phi) \definedby \fun a g \act  \phi(\inv g\act a)
  \). Note that here the symmetry $g$ is independent of the input $a$,
  in contrast to the \WLOG{} construction in which the symmetry is
  determined by the input $a$.


One advantage of topologically sorted DAGs is that one can compute the
single-source shortest paths in linear time simply by processing the
vertices in the topological order. Let us use the \WLOG construction
to make this explicit.

\paragraph{Group action}
Let $\Graph n$ be the set of all directed graphs on $n$ vertices,
which we represent as binary relations on $\Fin n \definedby \set{0, 1, \ldots, n-1}$,
relating two vertices if there is an edge between them. Then, the
symmetric group $\Sym n$ acts on a graph $\D \in \Graph n$ by
permuting the vertices:
\[
  i \to_{\perm \act \D} j \iff \inv\perm \, i \to_{\D} \inv\perm \, j
\]
For example, here is an action of a permutation that topologically sorts a DAG:
\[
D \definedby
  \begin{tikzpicture}[baseline=(current bounding box.center), scale=0.8,yscale=.5]
    \begin{scope}
      \node (a) at (0,2) {$1$};
      \node (b) at (2,2) {$3$};
      \node (c) at (0,0) {$0$};
      \node (d) at (2,0) {$2$};
      \node (e) at (4,2) {$5$};
      \node (f) at (4,0) {$4$};

      \draw[->] (a) -- (b);
      \draw[->] (a) -- (c);
      \draw[->] (b) -- (d);
      \draw[->] (c) -- (d);
      \draw[->] (b) -- (e);
      \draw[->] (d) -- (f);
      \draw[->] (e) -- (f);
    \end{scope}

    \begin{scope}[xshift=8.5cm]
      \node (a) at (0,2) {$0$};
      \node (b) at (2,2) {$1$};
      \node (c) at (0,0) {$2$};
      \node (d) at (2,0) {$3$};
      \node (e) at (4,2) {$4$};
      \node (f) at (4,0) {$5$};

      \draw[->] (a) -- (b);
      \draw[->] (a) -- (c);
      \draw[->] (b) -- (d);
      \draw[->] (c) -- (d);
      \draw[->] (b) -- (e);
      \draw[->] (d) -- (f);
      \draw[->] (e) -- (f);
    \end{scope}
  \end{tikzpicture}
  =
  \begin{psmallmatrix}
    0 & 1 & 2 & 3 & 4 & 5 \\
    2 & 0 & 3 & 1 & 5 & 4
  \end{psmallmatrix} \act \D
\]
This action is the exponential
action $(\Fin n)^2 \to \Bool$, where the action on the domain is
the product of the permutation $\Sym n$-action on $\Fin n$ with itself, and the
codomain action is the trivial one.

Recall that a \emph{walk} $w : i_0 \walkto i_{n-1}$ of length $\length w =
n$ is a sequence
\(
  i_0 \to i_0 \to i_1 \to \cdots \to i_{n-1}
\) of $n$ compatible edges.
The \emph{distance} between two vertices
in a graph
\(
  \dist(\D) : (\Fin n)^2 \to \naturals\union\set\infty
\) is the length of the shortest walk between them \(
  \dist(\D)(i,j) \definedby \min_{w : i \walkto j} \length w
\).
If there are no walks $i \walkto_{\D} j$, then $\dist(\D)(i, j) = \infty$.
%
Every walk $i \walkto_{\perm\act \D} j$ in the permuted graph $\perm
\act \D$ corresponds to a walk $\inv\perm i \walkto_{\D} \inv\perm j$
in the original graph $\D$. Since this action does not change the
length of the path, we have that $\dist(\perm \act \D)(\perm i,
\perm j) = \dist(\D)(i, j)$.

We equip the set of distance functions $\Dist n \definedby (\Fin
n)^2 \to \naturals\union\set\infty$ with the $\Sym n$-action given by
\(
  (\perm\act f)(i, j) = f(\perm \, i, \perm \, j)
\).
This action is the exponential of the product action on
$(\Fin n)^2$ and the trivial action on $\naturals\union\set\infty$.
The preservation of distances under permutation is exactly the
equivariance of the function
\(
  \dist : \Graph n \equito \Dist n
\).

Let $\Dag n \subseteq \Graph n$ be the set of all those
relations whose transitive closure is irreflexive, meaning there is
no cycle $i_0 \to i_1 \to \cdots \to i_k \to i_0$. We can lift
the permutation action to DAGs along this inclusion: $(\act) : \Sym n \times \Dag n \to
\Dag n$, since any cycle $i \walkto_{\perm\act \D} i$ in the
permuted graph would imply a cycle $\inv\perm i \walkto_{\D}
\inv\perm i$ in the original DAG $\D$. Therefore, restricting the distance
function along this inclusion gives an
equivariant function \(
  \dist : \Dag n \equito \Dist n
\).


\paragraph{Canoniser}

Each DAG can be topologically sorted, giving us a map $\topSort : \Dag
n \to \Sym n$ such that $\topSort \D \act \D$ is topologically
sorted~\cite{cormen}. Each canonical element is therefore a
topologically sorted graph. However, without additional assumptions on
the sorting algorithm, such as that the immediateness property of
\appref{normalisers}, not all topologically sorted graphs are
necessarily canonical. The standard depth-first search algorithm
for topological sorting is immediate in this sense~(cf.~\exampleref{normal sorting} in \appref{normalisers}) and so
its set of canonical DAGs is exactly the topologically sorted DAGs.

\paragraph{Core function}
For each graph $\D \in \Graph n$, the distance function satisfies the recurrence formula:
\[
  \dist(\D)(i,j) =
  \begin{cases}
    0 & (i = j) \\
    1 + \min_{j' \to_{\D} j} \dist(\D)(i, j') & \text{otherwise}
  \end{cases}
\]
When $\D$ is a topologically sorted DAG, we have $j' \to_{\D}j$
only if $j' < j$. Hence, we can use the above recurrence to define a
total function $d(\D)$, as the second argument strictly decreases:
\[
  d(\D)(i,j) =
  \begin{cases}
    0 & (i = j) \\
    1 + \min_{j' \to_{\D} j} d(\D)(i, j') & \text{otherwise}
  \end{cases}
\]

\paragraph{The \WLOG construction}

Usually, when defining the distance function on a DAG, one assumes
that the graph is already topologically sorted. We explicate this
assumption by extending $d$ to all DAGs as $\wlg(\topSort, d) : \Dag n
\to \Dist n$. This extension is an instance of \WLOG{} because we need to
transform both the input and the output using the same symmetry.
We already know that $d$ coincides with $\dist$ on
topologically sorted DAGs. Let us see that $\wlg(\topSort, d)$ does
the same, but for all DAGs. Take $\D \in \Dag n$, abbreviate $\perm_{\D}
\definedby \topSort \D$, and compute:
\[
  \wlg(\topSort, d)(\D)
  \explain={by definition of $\wlg$}
  \inv-{\perm_{\D}} \act d(\perm_{\D} \act \D)
  \explain={$d$ and $\dist$ coincide\\[-5pt]on $\Canon\topSort$}
  \inv-{\perm_{\D}} \act \dist(\perm_{\D} \act \D)
  \explain={$\dist$ is equivariant}
  \inv-{\perm_{\D}} \act \perm_{\D} \act \dist(\D)
  \explain={group action axioms}
  \dist(\D)
\]
