# Supplementary material for: Mathematical foundations for symmetric programming and reasoning
Source: arXiv:2611.17106 source file (2026-11-12)
Supplement: Supplementary file 3 [file dijkstra.tex]

\section{Dijkstra's analysis}

\citeauthor{dijkstra:wlog} argues against extant usage of \WLOG{}
reasoning.  He does not define the principle in general, but uses as
example two predicates on unordered pairs which he formulates as two
predicates on ordered pairs $\phi,\psi : \A^2 \to \Prop$ with the
property:
\begin{enumerate}
\item\label{dijkstra 0}
  $(\x,\y) : \A^2 \types \phi(\x,\y) = \phi(\y,\x)$ and
  similarly for $\psi$.\\
\end{enumerate}
He deconstructs a \WLOG{} argument
as consisting of two arguments:
\begin{enumerate}[resume]
\item\label{dijkstra 2}
  finding a third predicate $\xi : \A \to \Prop$ such
that $(\x,\y) : \A^2 \types \phi(\x,\y) \land \xi \x \implies \psi(\x,\y)$.
\item\label{dijkstra 5}
  showing that $\phi(\x,\y) \implies (\xi \x \lor \xi \y)$;\\
\end{enumerate}
and concluding that, \WLOG, $\phi(\x,\y) \implies \psi(\x,\y)$.
He also asserts that, when the \WLOG{} argument was presented, or justified,
to him,
it also included this step:
\begin{enumerate}[resume]
\item\label{dijkstra 3}
  stating that `by similar reasoning,
  $(\x,\y) : \A^2 \types \phi(\x,\y) \land \xi \y \implies \psi(\x,\y)$'
\end{enumerate}
He then argues that mathematicians employing this principle in practice:
do not show (\ref{dijkstra 5}) explicitly; and do not
carefully explain the symmetry, i.e., that $\phi(\x,\y) = \phi(\y,\x)$
and similarly $\psi$ are predicates over unordered pairs. Moreover, he
argues that arguing for step (\ref{dijkstra 3}) unnecessary. It follows
from steps (\ref{dijkstra 0}) and (\ref{dijkstra 5}), or
better: if we phrased $\phi$ and $\psi$ as predicates over unordered
pairs directly, we will notice that step (\ref{dijkstra 3})
and step (\ref{dijkstra 2}) are the same statement.

First, lets see how his \WLOG{} principle, formulated as steps
(\ref{dijkstra 0}--\ref{dijkstra 5}), is an instance of our \WLOG{}
principle. We work under the context $\Ctx \definedby (\x,\y) : \A^2,
\phi(\x,\y)$.  Step (\ref{dijkstra 0}) shows we deal with invariant
predicates for the $\Sym 2$-action over $\A^2$ that swaps $\x$ with
$\y$. Define the indexed canoniser, which uses step (\ref{dijkstra
  5}), by $\canoniser(\ma,\mb) \definedby \stet$ when $\xi \ma$ and
$\canoniser(\ma,\mb) \definedby \swap$ when $\xi \mb$. Thus in
canonical elements, the first component satisfies $\xi$.  Step
(\ref{dijkstra 2}) provides the core function.

We agree with his analysis that steps (\ref{dijkstra 5}) and
(\ref{dijkstra 0}) are typically implicit. Since \WLOG{} is typically
used as a recipe with these steps left implicit, it is not clear what one should
show in each instance.  In contrast, our proposed \WLOG{} principle is
general and precise. It draws attention to group actions, canonisers,
and canonical elements. While managing the actions at play is subtle,
there is no doubt about the appropriate proof obligations.

Lets turn to his final point, arguing against step (\ref{dijkstra
  3}). This point is more nuanced, and possibly in the remit of
philosophers or historians of mathematics, as it concerns analysing
exactly what Dijkstra meant or objected to. While Dijkstra's logical
reasoning is sound, we do see some value in the practice of explaining
exactly how the symmetric argument goes, in light of our revised
\WLOG{} principle. If both the action and the canoniser are left
implicit, one is in the dark about why the canonical case is canonical
at all. Lacking a formal and general \WLOG{} principle to appeal to,
the presenters explaining how symmetric cases go help us recover the
action and the canoniser.
