# Supplementary material for: Mathematical foundations for symmetric programming and reasoning
Source: arXiv:2611.17106 source file (2026-11-12)
Supplement: Supplementary file 4 [file harrison.tex]

\section{Case study I: Harrison's tactics}
\applabel{shur's inequality}
We now present the case study we summarised in \subsecref{mathematical
  reasoning wlog} concerning Harrison's seminal
paper~\cite{DBLP:conf/tphol/Harrison09} which develops a suite of HOL
tactics for simplifying proof obligations using
with-out-loss-of-generality arguments. We try to recover those using our
proposed \WLOG{} principle. We succeed in four out of five tactics, some
times improving on Harrison's development. Notably, one of Harrison's
tactics does not readily instantiate our \WLOG{} principle, as we will
discuss.

\subsection{Summary}

In his seminal paper, \citet{DBLP:conf/tphol/Harrison09} develops a
suite of HOL tactics for simplifying proof obligations using
with-out-loss-of-generality arguments. In \appref{shur's inequality}
we summarise a case study: whether and how we can recover those tactics using
a single \WLOG{} principle. We can recover four out of his five
\WLOG{} tactics. In the cases we can recover, our \WLOG{} principle
improves on Harrison's work in the following conceptual way.

Harrison argues that \WLOG{} is a separate logical principle, rather than
a short-hand for checking the different permutations of the assumptions.
For example, Harrison's \eqref{harrisons:wlog3} principle lets us
represent the proof for Schur's inequality more faithfully. Interestingly,
his development shifts the combinatorics involving the different cases
from the proof of the original proposition to the proof
of the principle~\eqref{harrisons:wlog3}. We improve on Harrison's proof and
transfer this burden entirely to general group-theoretic results involving
the two permutations $(1\,2)$ and $(1\,3)$ that generate
the symmetric group $\Sym 3$. Neither the example nor the principle nor its proof
involve combinatorics.

Apart from Schur's inequality, Harrison develops four tactics for
\WLOG{} reasoning in geometry. The tactics use a bank of results about
invariance and equivariance of various operations under
translations and orthonormal transformations.
Of the four tactics, three are immediate special cases of our wlog
principle, as we show in \appref{shur's inequality}.

Notably, one of Harrison's tactics does not readily instantiate
our \WLOG{} principle.
This dimensionality reduction tactic states that a property of points
in $\reals^3$ that only concerns coordinates in the $\x$-$\y$ plane,
can be proved \WLOG{} of points in $\reals^2$, so long as we modify the
property to first embed the points into $\reals^3$:
\[
\tag{pad2d3d\_tac}
\inferrule{
  \forall (\x,\y) : \reals^2. P(\x,\y,0)
}{
  \forall (\x,\y,\z) : \reals^3. \z = 0 \implies P(\x,\y,\z)
}
\]
(An inference-rule presentation unfortunately de-emphasises its
importance for goal-simplification.)

This principle is of quite different nature than the other \WLOG{}
principles, to the point where we think it should not be classified
as a \WLOG{} principle. It seems more appropriate to think of it as
a reduction, rather than reasoning \WLOG{}
% No period is missing here, as WLOG ends with a dot.
In that sense, our work is
revisionist: we do not account for all previous principles named \WLOG{},
but instead we revise some of them based on a crisp criterion:
instantiation as a general unifying \WLOG{} principle.

The concepts of `equivariance' and `group actions' are not explicit in
Harrison's development. However, many of the intermediate results he
uses are, in fact, equivariance results. For example, that the angle
between three points is invariant under orthogonal transformations is
the equivariant function $\mathsf{angle} : (\reals^3)^3 \equito
\oc{-\pi}{\pi}$, or that the cross product of vectors is equivariant
under rotations $(\cross) : (\reals^3)^2 \equito
\reals^3$. Interestingly, Harrison concludes by considering a hypothetical
reflection library that for general
\WLOG{} reasoning. He values the benefit of
working generally, but warns against limited the situation so that
only propositions expressible in the reflected syntax may be
used. Grounding \WLOG{} reasoning with group actions negotiates these
constraints differently: the framework of group actions gives
generality and the ability to develop a meta-theory. At the same time, group actions
are sufficiently open-ended and extensible that the framework does not limit the
development to one specific application domain such as geometric
reasoning.

Before concluding, we emphasise that merely expressing Harrison's \WLOG{}
tactics with our \WLOG{} principle does not account at all to the overall
structure of the \WLOG{} library in HOL. For example, Harrison invested
effort in developing other auxiliary tactics and proof engineering
that allow a high degree of automation when employing these
principles.

\subsection{Schur's inequality}
Harrison introduces the following principle\footnotemark{}
\eqref{harrisons:wlog3} which states that it is sufficient to show
permutation invariant propositions only for sorted triples~\cite[page
  44]{DBLP:conf/tphol/Harrison09}:
\begin{align*}
  \tag{$\wlg_3$}
  \label{harrisons:wlog3}
  \inferrule{
    \forall \x,\y,\z : (0,\infty).P(\x,\y,\z) \Rightarrow P(\y,\x,\z) \land P(\x,\z,\y)\\\\
    \forall \x,\y,\z : (0,\infty).\x \le \y \land \y \le \z \Rightarrow P(\x,\y,\z)
  }{
    \forall \x,\y,\z : (0,\infty).P(\x,\y,\z)
  }
\end{align*}
\footnotetext{Available here: \url{https://github.com/jrh13/hol-light/blob/master/int.ml\#L612} .}


\begin{example}\examplelabel{schur's inequality actions}
  Define Schur's inequality as the function
  $\Schur : \DFun{\x_0, \x_1, \x_2,\BoundV t}{(0,\infty)} \Prop$:
  \[
  \Schur(x_0, x_1,x_2, t) \definedby
  0 \leq x_0^{t}(x_0-x_1)(x_0-x_2)+x_1^{t}(x_1-x_2)(x_1-x_0)+x_2^{t}(x_2-x_0)(x_2-x_1)
  \]
  Equipping $\Ctx \definedby (\x_0, \x_1, \x_2,\BoundV t :
  (0,\infty))$ with the $\Sym 3$-action that permutes the first
  three components, and $\Prop$ with the trivial $\Sym 3$-action, we
  have that Schur's inequality is an equivariant function between
  (non-indexed) sets $\Schur : \EFun{\x_0, \x_1,
    \x_2}{(0,\infty)}\Prop$. This fact means that the associated
  family $\Ctx \types \Schur(x_0, x_1,x_2, t)$ is a $\Ctx$-indexed
  action. Moreover, any proof term of Schur's inequality $\Ctx \types
  p : \Schur(x_0, x_1,x_2, t)$ is equivariant.
\end{example}

The purpose of \eqref{harrisons:wlog3} is to prove $\forall
\x,\y,\z : (0,\infty).  P(\x,\y,\z)$. Under the Curry-Howard
correspondence, it amounts to a dependent function $p :\DFun{\x,\y,\z}
{(0,\infty)^3}{P(\x, \y, \z)}$ for some proposition $P : (0,\infty)^3
\to \Prop$. To apply the wlog construction, we need to equip
both the domain $(0,\infty)^3$ and the codomain $P$ with an action, as
we have done in \exampleref{schur's inequality actions}, i.e.,
that $P$ is invariant.

\OhK{I moved material about generators from here to the dependent types appendix.}

Thus, the top assumption in \eqref{harrisons:wlog3} ensures $P :
(0,\infty)^3 \to \Prop$ is invariant.

Here, we can see the reduction of the number of cases we need to
consider. Even though the symmetric group~$\Sym n$ has $n!$ elements,
it can be generated from far less, for example a single cycle $(1 \, 2
\, \cdots \, n)$ and any transposition of adjacent elements, for
example $(1 \, n)$. For $\Sym 3$, the two transpositions $(1\,2)$ and
$(1\,3)$ also generate it.  Thus, to prove the invariance of $P$, we
need to consider only two cases.

Finally, to complete the construction, choose the unique sorting
function as the canoniser, and we need to provide a map $f : \DFun{\x,
  \y, \z}{\Canon{\sort}}{P(x, y, z)}$.  As we have established
earlier, the canonical elements for storing are exactly the sorted
tuples $\x \le \y \le \z$, so this map corresponds exactly to the
second assumption in~\eqref{harrisons:wlog3}.

Note the only combinatorics we have used are that $(1\,2)$ and
$(2\,3)$ generate $\Sym 3$. On a technical level, this is only a minor
improvement on Harrison's proof for \eqref{harrisons:wlog3}. On a
conceptual level, we have isolated the combinatorics to a well-known
fact about $\Sym 3$, and nowhere do we generate repetitive
cases. Moreover, we have used a general \WLOG{} principle, rather than a
bespoke one.

\subsection{Geometric equivariance}
Let us turn to Harrison's remaining four tactics\footnotemark{} for
wlog reasoning in geometry.
\footnotetext{Available here: \url{https://github.com/jrh13/hol-light/blob/master/Multivariate/wlog.ml} .}
The first tactic uses equivariance under
translation~\cite[Sec.~3]{DBLP:conf/tphol/Harrison09}:
\[
\tag{wlog origin}
\label{wlog origin}
\inferrule{
  \forall \ma, \x : \reals^n. P(\ma + \x) \iff P(\x)\\
  P(\vec 0)
}{
  \forall\x : \reals^n. P \x
}
\]
This is a special case for the action of the group of vector addition
$\seq{\reals^n, (+), \vec 0, (-)}$ on tuples of vectors. The canoniser
chooses the inverse $\canoniser v \definedby - v$,
making $\x = \vec 0$ the only canonical input.

His next couple of tactics use equivariance under the group of
orthogonal transformations of
$\reals^n$~\ibid[Sec.~5]{DBLP:conf/tphol/Harrison09} and its subgroup
of rotations. The next tactic embodies wlog reasoning where the input
vector is a non-negative multiple of some fixed non-zero vector $v_0$:
\[
\inferrule{
  \forall \BoundV f : \transformation, \x : \reals^n. P(\BoundV f\, \x) \iff P \x\\\\
  v_0 \neq \vec 0\\
  \forall t : (0,\infty). P(t v_0)
}{
  \forall \x : \reals^n. P\x
}
\tag{geom\_basis\_multiple\_tac}
\]
This is a special case of our \WLOG{} principle where the canoniser provides a
symmetry that reorients the input vector $\x$ with $v_0$, for example
through translation by the angle between them.

The next tactic concerns properties of planes in $\reals^3$, given as
$\set{\x \suchthat \x \bullet v_0 = d}$ for $v_0 \neq \vec 0$, and
reasons that \WLOG{} the plane is $\set{\x \suchthat \x \bullet (0, 0, 1) =
  0}$, i.e., the plane is the $\x$-$\y$ plane
$\set{(x,y,0) \suchthat x,y \in \reals}$:
\[
\tag{geom\_horizontal\_plane\_tac}
\inferrule{
  \forall \BoundV f : \transformation, \BoundV p : \plane.
    P(\BoundV f\, \bracks{\BoundV p}) \iff P \BoundV p\\\\
  P\set{(x,y,0) \suchthat x,y \in \reals}
}{
  \forall \BoundV p : \plane. P\,\BoundV p
}
\]
This is a special case of our \WLOG{} principle where the group is the
subgroup of automorphisms of $\reals^3$ generated by translations and
orthogonal transformations of $\reals^3$. The canoniser rotates the
plane so that $v_0$ has the same direction as $(0,0,1)$, and
translates it so that it coincides with the $\x$-$\y$ plane.
The code-base contains a similar tactic for rotating a Euclidean space
so that a given line becomes the $\x$-axis.
