# Supplementary material for: Mathematical foundations for symmetric programming and reasoning
Source: arXiv:2611.17106 source file (2026-11-12)
Supplement: Supplementary file 5 [file normality.tex]

\section{Weak normalisers}
\applabel{weak normalisers}

\OhK{Probably remove?}

We call elements with indistinguishably neutral norm \emph{weakly
normal}: $\cnorm[\canoniser]a \stabeq a \unit$, and define the
\emph{weak kernel} as the set of weakly normal elements $\WKer
\canoniser \definedby \set{a \in \carrier\A \suchthat
  \cnorm[\canoniser] a \stabeq a \unit}$.  Every normal element is
weakly normal, but there may be more weakly normal elements. For
example, in a canoniser for binary trees that assigns $\canoniser'
\Leaf \definedby \swap$, the leafs are weakly normal, but not
normal. Similarly, in a canoniser for plane rotations that sends the
origin to a non-trivial rotational symmetry, the origin is weakly
normal but not normal.

A canoniser is \emph{weakly normal} when every canonical element is
weakly normal. Since more elements may be weakly normal,
i.e.~$\Ker\canoniser \subset \WKer\canoniser \subset
\Canon\canoniser$, a canoniser may be weakly normal even if it is
not normal.

\begin{lemma}\lemmalabel{equivariant canoniser weakly normal}
  An equivariant canoniser is weakly normal.
\end{lemma}

\begin{proof}[of \lemmaref{equivariant canoniser weakly immediate}]%
  Calculate:
  \[
  \canoniser(\canoniser a \act a) \stabeq{\canoniser a \act a}
  \canoniser a \mul \inv{\canoniser a} = \unit
  \tag*{\qedhere}
  \]
\end{proof}
