# Supplementary material for: Mathematical foundations for symmetric programming and reasoning
Source: arXiv:2611.17106 source file (2026-11-12)
Supplement: Supplementary file 6 [file poc-implementation.tex]

\section{Proof-of-Concept: removing performance overheads for symmetric data types}
\applabel{poc implementation}

In \subsecref{partial evaluation} we described techniques for removing
some of the performance overhead incurred by symmetric programming
when projecting a subtree. There, we used the free action construction
and the symmetric strength. A skeptical reader may doubt whether these
techniques indeed remove the performance bottleneck. While this is the
topic of future work, we include a preliminary experiment
demonstrating that these techniques indeed remove the bottlenecks, and
are feasible even for the dependently-typed setting.

We use Idris~2~\cite{DBLP:conf/ecoop/Brady21}, a dependently-typed
programming language. We implemented a dependently-typed version of
the subtree projection function from \exampleref{subtree projection}.
Idris~2 implements a version of McBride and
\citeauthor{atkey:quantitative-type-theory}'s \emph{quantitative type
theory}~\cite{atkey:quantitative-type-theory}. It allows us to ensure
some values must be erased at runtime. We erase indices in
indexed actions. Some functions, such as subtree projection, in fact
require this index, and so we use a singleton type. We implemented
three functions of the type:
\[
t : \Tree \types
\subtree : \TreePath\, t \equito \parent{\set t \to \Tree}
\]

The function requires little computation, and so most of the
computational complexity concerns the overhead of deconstructing the
path and the tree, and projecting out the result. The baseline
implementation includes both $\Lft\::p$ and $\Rgt\:: p$ cases
explicitly.  The naive implementation uses symmetric programming to
remove the symmetric case $\Rgt\:: p$, but in turn flips the input
tree given via the singleton, and the result. The optimised
implementation employs dependently-typed counterparts to the
performance engineering techniques from \subsecref{partial
  evaluation}.  The benchmarks construct a tree of depth $d$ for
$d=11$ (including the naive implementation) and $d=10,000$ (excluding
the naive implementation), and then run each implementation for all
paths of length $0 \leq \cardinality p < d$. We use alternating paths
of the form $\Rgt\:: \Lft\:: \cdots \:: \Nil$ to make the symmetric
programming tests flip both inputs and outputs in every recursive
call. For simplicity, we only used the generic action for the
$\TreePath$ indexed symmetric data type, and did not use a generic
action for the simply-typed $\Tree$. The optimised implementation did
use the $\Sym2$-strength for the functor $F_{\Tree} : \Set \to \Set$
when deconstructing the tree alongside the path. The test harness does not
isolate the measurements from the interference of garbage collection.


\figfile{poc-images}{Proof-of-concept: Idris~2 dependently-typed subtree projection
  implementations. The baseline implementation includes redundant symmetric cases,
  the naive implementation flips the tree repeatedly, and the optimised implementation uses the free action and strength to remove the performance bottlenecks.
  (a) runtimes on a tree of depth 11, projecting subtrees of depth 0--10;  (b)
  runtimes of baseline and optimised benchmarks on a tree of depth 10000; and
  (c) log-runtime of the benchmark from (b).}

\figref{poc-images} presents sample runtimes from an HP EliteBook 640 14 inch G11
Notebook PC with Intel Core Ultra 5 135U$\times$14, 32.0GiB memory,
running Ubuntu 24.04.3 LTS. \figref{poc-images}(a)
plots the runtimes of the three benchmarks on a tree of depth $d =
11$. While the naive implementation can cope with trees of depth
larger than $d = 11$, the difference in performance to the baseline
and optimised implementation is so large that they are indiscernible
in the resulting diagram, and having the paths run up to length $10$
is a nice round number. As we can see, the naive test indeed incurs
several orders of magnitude of overhead, and the optimised version
removes much of this overhead.  The shape of the naive test runtime
curve may seem surprising, and we suggest partial explanations below.

\figref{poc-images}(b) plots the runtimes of baseline and optimised
tests for a larger tree of depth $d=10,000$. The test that uses
symmetric programming still incurs overhead. \figref{poc-images}(c)
plots the same data against a log scale to gauge whether
this overhead changes the asymptotic runtime. The two graphs seem to
have similar shapes, suggesting the techniques of \subsecref{partial
  evaluation} remove the asymptotic overhead.

We explain the shape of the naive test's runtime as follows. The path
of length $0$, $\Nil$ incurs no tree flipping, returning the input
tree immediately. Accordingly, the test has similar runtime to the
other tests. Every recursive call with tree $t$, flips the tree $t$
and the result $s$. The longer the path, the smaller the result $s$.
For the path of length $1$, we flip a tree of depth $11$ on the input
and a tree of depth $10$ on the output. For the path of length $2$, we
flip a tree of depth $11$ and a tree of depth $10$ on the input, but
flip a tree of depth $9$ twice on the output. And so on. This account
does not incorporate the overhead of memory allocation.  The initial
tree representation shares the same subtree for both children at every
node. Once the naive implementation starts flipping the tree, this
sharing is lost, incurring a large memory footprint, and potentially
spends some time on garbage collection. This may have averaging
effects on the curve. Further experimentation and analysis are needed
to fully explain the curve.

We conclude with some qualitative analysis of the experiment. While
the symmetric code never considers redundant symmetric cases, it
requires substantial infrastructure. Much of the symmetric programming
code is, however, shared between the two benchmarks: the structure
functors, their strength, their canonisers, and relevant
\citeauthor{mcbride-mckinna:views} views~\cite{mcbride-mckinna:views}
for convenient pattern-matching on the canonical elements. This
suggests that additional examples could amortise the cost of the
development. Further experimentation should also identify the right
programming abstractions to alleviate layers of nested pattern
matching and Idris~2 specific plumbing.
