# Supplementary material for: Mathematical foundations for symmetric programming and reasoning
Source: arXiv:2611.17106 source file (2026-11-12)
Supplement: Supplementary file 7 [file supplementary-preamble.tex]

\setboolean{WithSupplementary}{true}
